# Supplementary material for: Self-Employment as a Career Investment
Source: arXiv:2509.01265 ancillary file (2026-11-15)
Supplement: Supplementary file 1 [file SelfEmployment_CareerConcerns_slides.pdf]

# Self-Employment as a Signal: Career Concerns with Hidden Firm Performance

Konstantin Popov   Georgy Lukyanov   Shubh Lashkery

September 5, 2025

# Outline

Motivation and question

Model

Benchmark and equilibrium posting

Illustration

Empirical implications

Extension: worker learning

Discussion and wrap-up

# Motivation

- ▶ Markets often see some but not all output: portfolios, ratings, commits (public) vs. most inside-firm performance (hidden).
- ▶ Workers face an **insurance–information trade-off**: hidden employment insures today; public output builds portable reputation.
- ▶ We ask: *When do workers choose hidden employment forever? How do wages respond when firms infer from applications?*

## What we do

- ▶ Dynamic choice each period: **Self-employment** ( $S$ ) with public Bernoulli outcome; **Hidden employment** ( $E$ ) with flat wage.
- ▶ Public belief tracked by a  $\text{Beta}(\alpha, \beta)$  posterior;  $S$  updates  $(\alpha, \beta)$ ,  $E$  leaves it unchanged.
- ▶ Two posting regimes:
  - ▶ **Benchmark (myopic)**: wage equals public mean  $w^B(\alpha, \beta) = \mu(\alpha, \beta)$ .
  - ▶ **Equilibrium (inference-aware)**: wage equals mean talent of the *applicant pool*.

## Preferences, beliefs, and timing

- ▶ Risk-averse worker with increasing, concave  $u$ , normalized  $u(0) = 0, u(1) = 1$ ; discount factor  $\delta \in (0, 1)$ .
- ▶ Talent  $\theta \in [0, 1]$  (ability) is fixed; public belief is  $\text{Beta}(\alpha, \beta)$  with mean  $\mu = \alpha/(\alpha + \beta)$ .
- ▶ Each period: worker picks  $S$  or  $E$ ; outcome realized; public belief updates only under  $S$ ; wages are posted before the choice.

## Two value expressions

$$\begin{aligned}U_S(\theta; \alpha, \beta) &= \theta + \delta [\theta V(\theta; \alpha+1, \beta) + (1-\theta) V(\theta; \alpha, \beta+1)], \\U_E(\theta; \alpha, \beta) &= u(w(\alpha, \beta)) + \delta V(\theta; \alpha, \beta).\end{aligned}$$

- ▶ Define the gap  $\Delta(\theta; \alpha, \beta, w) \equiv U_S - U_E$ .
- ▶ **Single-crossing (Lemma):**  $\Delta$  is strictly increasing in  $\theta$  and strictly decreasing in  $w \Rightarrow$  cutoff behavior.

## Benchmark (myopic) wage posting

- ▶ Wage equals public mean:  $w^B(\alpha, \beta) = \mu(\alpha, \beta) = \alpha/(\alpha + \beta)$ .
- ▶ **Result (Absorption, benchmark):** If  $\theta \leq \hat{\theta}^B(\alpha, \beta)$  is willing to take  $E$  today, then  $E$  is optimal forever at  $(\alpha, \beta)$ .
- ▶ Intuition:  $E$  freezes the public state; the same comparison repeats next period.

## Equilibrium (inference-aware) posting

- ▶ Applicant pool under cutoff  $\hat{\theta}$ :  $[0, \hat{\theta}]$ . Posted wage is the *truncated mean*:

$$w^E(\alpha, \beta; \hat{\theta}) = \mathbb{E}[\theta \mid \theta \leq \hat{\theta}; \text{Beta}(\alpha, \beta)].$$

- ▶ **Fixed point for acceptance cutoff:**

$$\Delta(\hat{\theta}; \alpha, \beta; w^E(\alpha, \beta; \hat{\theta})) = 0.$$

- ▶ **Result (Existence & uniqueness):** unique  $\hat{\theta}^E(\alpha, \beta)$ . Intuition: truncated mean increases in  $\hat{\theta}$ ; indifference decreases in  $w$ .



## Benchmark vs. Equilibrium: wages and cutoffs

- ▶ At the same public state,  $w^E(\alpha, \beta; \hat{\theta}) \leq w^B(\alpha, \beta)$  (strict if  $\hat{\theta} < 1$ ).
- ▶  $\Rightarrow$  **Lower acceptance cutoff in equilibrium:**  $\hat{\theta}^E(\alpha, \beta) \leq \hat{\theta}^B(\alpha, \beta)$ .
- ▶ Economic consequence: fewer mid-types accept hidden employment early; stronger selection into public production.

## Three-period example (very brief)

- ▶ Prior  $\text{Beta}(1, 1)$ ,  $u(x) = x^\rho$  with  $\rho \in (0, 1]$ .
- ▶ Last period: cutoff is  $u(w)$ . Benchmark wages:  $1/3, 1/2, 2/3$  at  $(1, 2), (1, 1), (2, 1)$ ; equilibrium wages are lower (pool pricing).
- ▶ Middle period ( $t=1$ ): equilibrium compresses success–failure wage gap (winner's-curse correction via application inference).

## Empirical implications

- ▶ Early careers: stronger types keep producing public signals (bigger belief moves from a single public outcome).
- ▶ Transitions into hidden employment spike after runs of low public realizations.
- ▶ With pool pricing, wage dispersion after public successes/failures is compressed relative to the myopic benchmark.
- ▶ Cross-occupation: more portable histories  $\Rightarrow$  more selection into public production and sharper wage responses.

## Extension: worker learns own type

- ▶ Worker has private posterior  $H_t$  with mean  $m_t$ ; public posterior mean  $\mu_t$  from the market.
- ▶ Choice is governed by a cutoff in private belief: take  $E$  iff  $m_t \leq \hat{m}(\alpha, \beta)$ .
- ▶ Absorbing logic persists locally:  $E$  freezes the *public* state; with flat wages,  $E$  remains optimal in a neighborhood of  $m_t$ .
- ▶ Equilibrium posting still discounts for selection; cutoffs shift accordingly.

## What to take away

- ▶ **Absorbing hidden employment:** when public beliefs are low, hidden employment is a self-confirming choice.
- ▶ **Equilibrium posting:** pool pricing yields a unique cutoff and tighter self-selection than the myopic benchmark.
- ▶ **Implications:** transparency policies and platform design can change the returns to public production.

## Selected references

- ▶ Holmström (1999), “Managerial Incentive Problems: A Dynamic Perspective.”
- ▶ Board & Meyer-ter-Vehn (2013), “Reputation for Quality.”
- ▶ Terviö (2009), “Superstars and Mediocrities: Market Failure in the Discovery of Talent.”
- ▶ MacLeod (2003), “Optimal Contracting with Subjective Evaluation.”

Thank you

Questions?
